# Supplementary material for: Epitaxial Strain-Dependence of Band Gaps in Oxynitrides compared to Oxides
Source: arXiv:1806.02050 source file (2018-06-06)
Supplement: Supplementary file 1 [file SupportingInformation.pdf]

# Supporting information for:
# Epitaxial Strain-Dependence of Band Gaps in Oxynitrides Compared to Oxides

Nathalie Vonrüti and Ulrich Aschauer
*Department of Chemistry and Biochemistry, University of Bern, Freiestrasse 3, CH-3012 Bern, Switzerland*
(Dated: June 5, 2018)

## S1. INFLUENCE OF HUBBARD U

As shown in figure S1 a, the band gap of $SrTaO_2N$ is almost unaffected by the magnitude of the Hubbard U correction applied on Ta *5d* states. $SrTaO_2N$ calculations were therefore performed without a Hubbard U correction (U=0). This is further justified by the independence of relative strain-dependent band-gap changes on Hubbard U as shown for the 5-atom high symmetry cell of $SrTiO_3$ in figure S1 b.

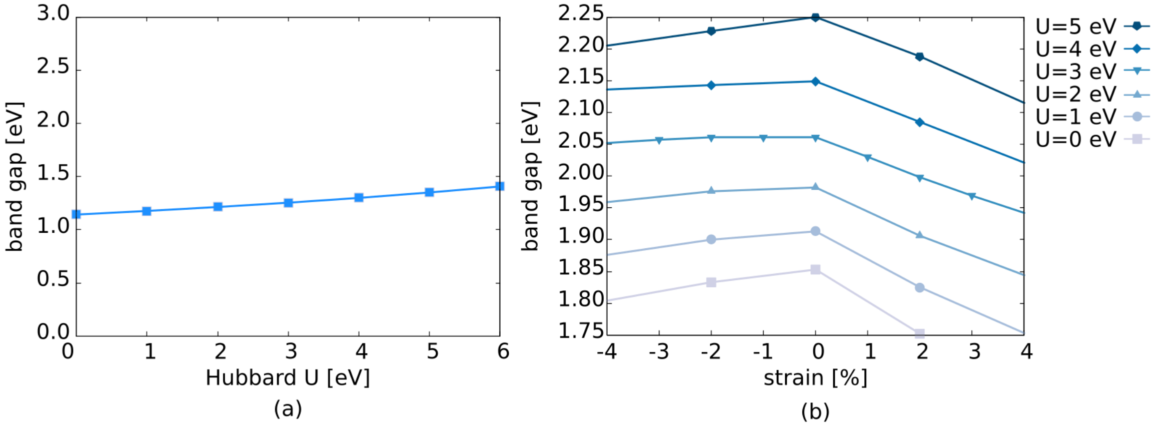


FIG. S1: (a) $SrTaO_2N$ GGA+U band gap as a function of Hubbard U. (b) Strain-dependent band gaps of $SrTiO_3$ for different Hubbard U values.

## S2. ANION ORDER IN $SrTaO_2N$ THIN FILMS

While we previously determined the strain-dependent energy for 8 different anion orders in $LaTiO_2N$[1], we here determine the detailed energetics in $SrTaO_2N$ only for the two anion orders (see figure 1) that were shown for $LaTiO_2N$ to be thermodynamically stable for strains between -4% and +4% strain. We start our relaxation calculations from the orthorhombic experimental structure[2] with a rotation pattern $a^-b^-c^+$. For the fully relaxed 40-atom unit cell we obtain the following lattice parameters: a= 8.18 Å, b= 8.18 Å, c= 7.95 Å. We designate structures as in our previous work by $a_s^b$, where $a$ denotes the anion order ($cis/trans$), $b$ the direction/plane along/in which the N-TM-N bonds are aligned and $s$ the strain plane. An example for the $cis_{bc}^{ac}$ structure is shown in figure S2. We find that under biaxial epitaxial strain in the $ac$ plane the $trans$ structure is stable for large compressive strain, whereas the $cis$ order $cis_{ac}^{bc}$ is stable from -5% to 1% strain and $cis_{ac}^{ac}$ is stable beyond 1% tensile strain (see figure S3).

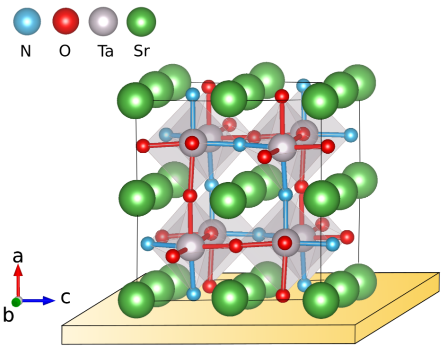


FIG. S2: Visualization of the used notation of the anion order and the strain plane: shown is the $SrTaO_2N$ $cis_{bc}^{ac}$ structure with Ta-N bonds in a and c direction and biaxial epitaxial strain applied in the bc plane.

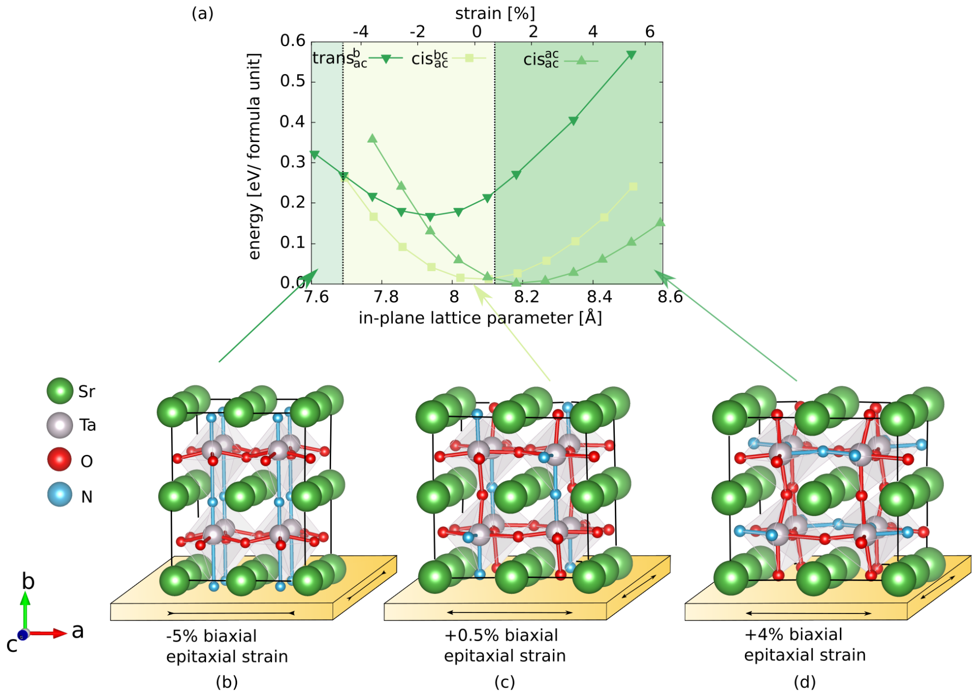


FIG. S3: (a) Total energy of epitaxially strained $SrTaO_2N$ as a function of the in-plane lattice parameter. Thermodynamically stable structures in the different strain regimes: (b) $trans_{ac}^{b}$ stable for compressive strain$_{\mathrm{ac}}$ larger than 5%; (c) $cis_{ac}^{bc}$ stable between -5% and 1% strain$_{\mathrm{ac}}$; (d) $cis_{ac}^{ac}$ stable for more than 1% tensile strain$_{\mathrm{ac}}$.

## S3. TOLERANCE FACTORS

The Goldschmidt[3] tolerance factor $t$ is commonly used to characterize the propensity of a perovskite to structural distortions. For oxides it is defined as

$$t = \frac{r_A + r_O}{\sqrt{2}(r_B + r_O)} \tag{1}$$

where $r_A$ and $r_B$ are the ionic radii of the A and B site respectively, whereas $r_O$ is the radius of oxygen. For our oxynitrides, we substitute the stoichiometric average of the oxygen and nitrogen radii for $r_O$:

$$r_O := \frac{2}{3} r_O + \frac{1}{3} r_N \tag{2}$$

Using this definition, we find similar tolerance factors for $LaTiO_2N$ (0.97) and $SrTaO_2N$ (0.98). In an oxide $t > 1$ implies an instability of the perovskite structure compared to hexagonal phases. A $t$ close to 1 suggests the presence of ferroelectric distortions, whereas with decreasing $t$ octahedral rotations become increasingly more favorable up to the point where the perovskite structure is no longer stable. This analysis suggests that $LaTiO_2N$ should have slightly larger octahedral rotations and smaller ferroelectric distortions compared to $SrTaO_2N$.

## S4. ROTATION ANGLES

We characterise the total magnitude of octahedral rotations by the sum of the average rotation angles in all 8 octahedra around the x, y and z axis:

$$\Theta = \frac{1}{8}\left(\sum_{i=1}^{8} \left(|\theta_{x,i}| + |\theta_{y,i}| + |\theta_{z,i}|\right),\right) \tag{3}$$

where $i$ is the index of the octahedron and $\theta_{x,i}$, $\theta_{y,i}$ and $\theta_{z,i}$ are the angles obtained by fitting a $X_1Y_2Z_3$ Tait–Bryan matrix to rotate the 6 TM-X bonds of each octahedron to lie along the pseudocubic axes. As shown in Figure S4, the total octahedral rotation magnitude $\Theta$ is smaller for all low energy anion orders of $SrTaO_2N$ compared to $LaTiO_2N$.

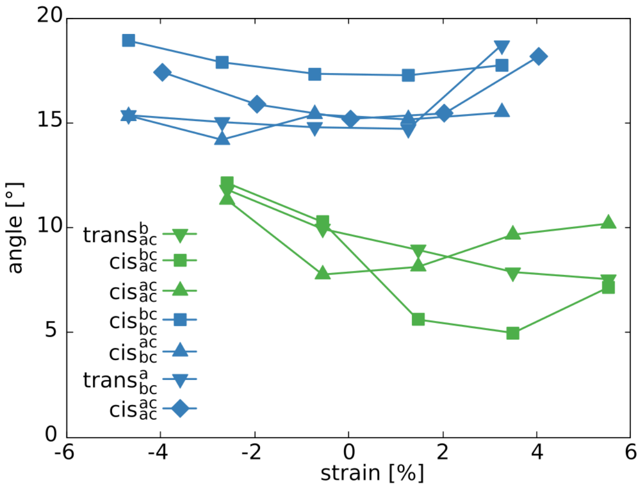


FIG. S4: Rotation angles of the different low energy structures of $LaTiO_2N$(blue) and $SrTaO_2N$ (green).

## S5. POLARITY

Previously, we determined the net polarization using Berry phase calculations[1]. Here we are however not interested in the overall polarization (which would be zero for an antipolar distortion) and we need a local observable for polarity that is moreover independent of the polarization direction. We use the ratio of consecutive TM-N bondlengths along a linear direction (i.e. N-TM-N) as an observable for polarity and subtract one from the obtained value. An observable of 0 thus indicates zero polarity. Using this observable we find that the polarization for $SrTaO_2N$ is generally larger than for $LaTiO_2N$ (see figure S5). Further, while $LaTiO_2N$ shows zero polarization for an intermediate strain range, $SrTaO_2N$ is polar over the whole strain range considered.

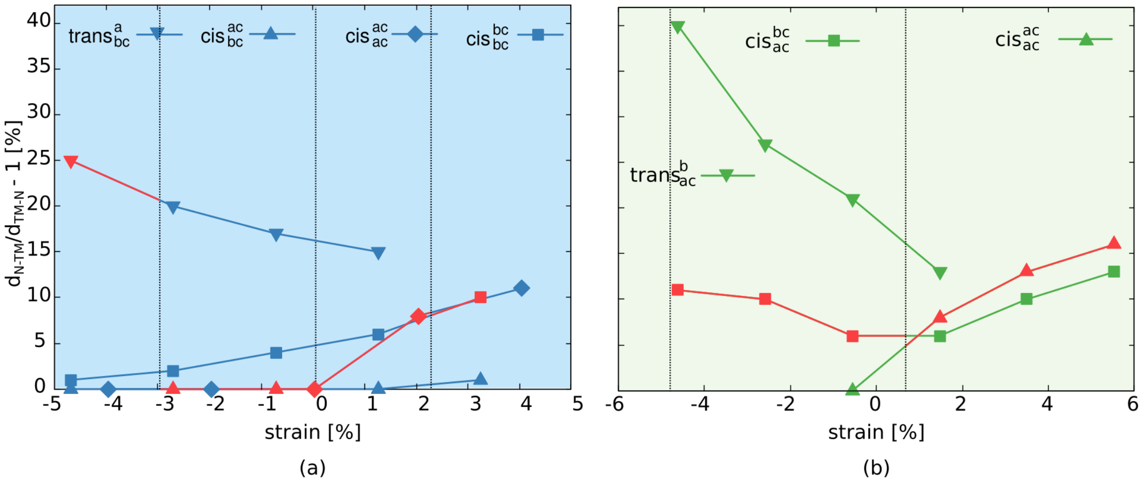


FIG. S5: Bondlength (d) based polarity observable $\frac{d_{N-TM}}{d_{TM-N}} - 1$ (0 indicating an non-polar structure) for (a) $LaTiO_2N$ and (b) $SrTaO_2N$. The vertical dashed lines indicate borders between strain ranges for which a certain structure is stable. The polarity of the most stable structure in a specific strain range is colored red.

## S6. FATBANDS OF NON-POLAR STRUCTURES WITHOUT ROTATIONS

Fatbands (see figure S6 and S7) are shown for the 5-atom high symmetry structures to support the sketch in figure 4 (b) and (c) in the main text.

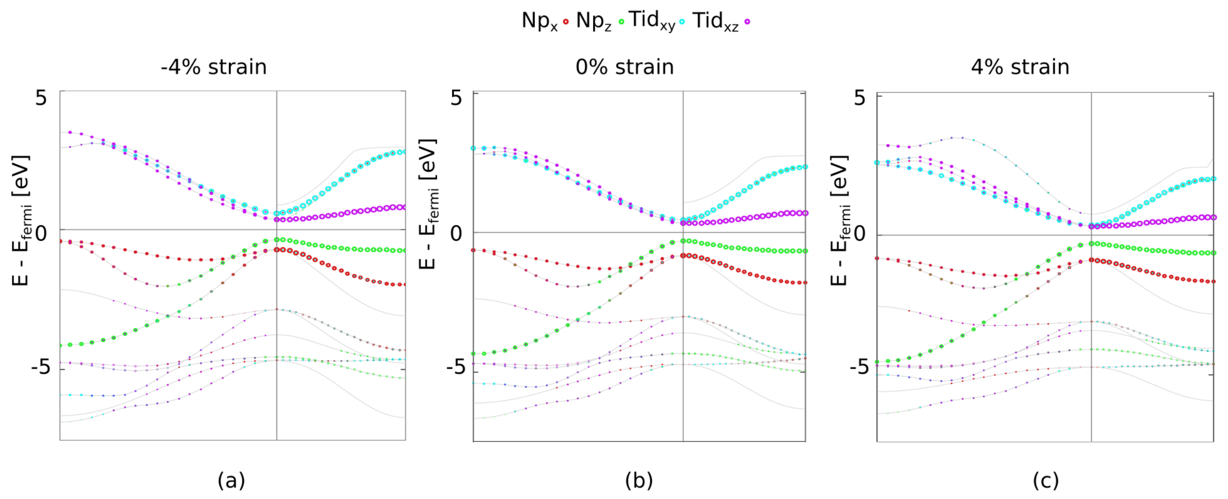


FIG. S6: Fatbands of non-polar *trans*-$LaTiO_2N$, without octahedral rotations at (a) -4% , (b) 0% and (c) +4% biaxial epitaxial strain.

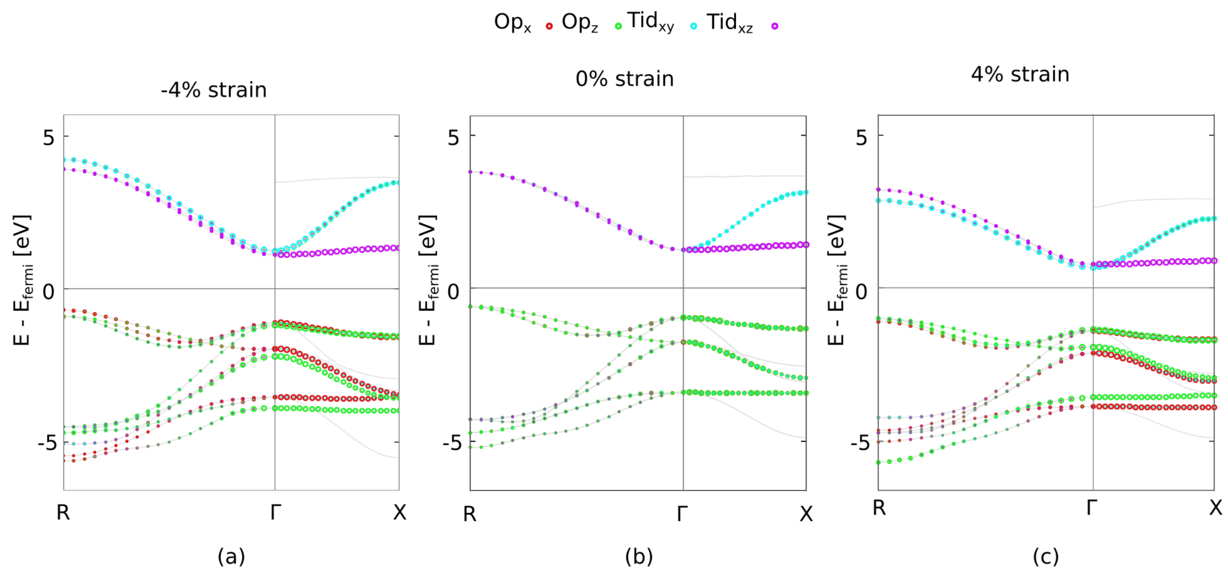


FIG. S7: Fatbands of non-polar $SrTiO_3$, without rotations at (a) -4% , (b) 0% and (c) +4% biaxial epitaxial strain.


[1] N. Vonrüti and U. Aschauer, Physical Review Letters **120**, 046001 (2018).
[2] S. J. Clarke, K. A. Hardstone, C. W. Michie, and M. J. Rosseinsky, Chemistry of materials **14**, 2664 (2002).
[3] V. M. Goldschmidt, Naturwissenschaften **14**, 477 (1926).
